# Supplementary material for: Vorticity and magnetic dynamo from subsonic expansion waves II: Dependence on magnetic Prandtl number, forcing scale, cooling time
Source: arXiv:2404.10804 ancillary file (2024-12-10)
Supplement: Supplementary file 1 [file Tables.pdf]

# Complete set of runs for *Vorticity and magnetic dynamo from subsonic expansion waves II*

The following tables contain the whole list of all simulations included in this article, as well as the most relevant runs in Elias-López et al. [2023] marked **violet**. Keep in mind that the runs from the past article do not have all diagnostics.

Table 1: Barotropic (i.e. isothermal) runs without shear. In every model we use  $B_0=10^{-6}$  as seed field, and the new runs all have  $\Delta t=0.02$  as interval between two different explosions.

| 256 <sup>3</sup> | $\nu$              | $\eta$             | $\Omega$ | $\phi_0$ | R          | $t_{tot}$ | $t_{turn}$ | $k_\omega/k_f$ | Re (Rm)       | Re $_\omega$ | $u_{rms}$                           | $u_{rot}/u_{tot}$  | $r(t_{turn}^{-1})$        | $r_\omega(t_{turn}^{-1})$ |
|------------------|--------------------|--------------------|----------|----------|------------|-----------|------------|----------------|---------------|--------------|-------------------------------------|--------------------|---------------------------|---------------------------|
| M_0W0.10         | 2·10 <sup>-4</sup> | 2·10 <sup>-4</sup> | 0        | 2.6      | 0.10       | 282.77    | 0.77       | 0.04158        | 16.15         | 0.671        | (6.458 ± 0.042) · 10 <sup>-2</sup>  | 0.019              | -                         | -                         |
| M_0W0.20         | 2·10 <sup>-4</sup> | 2·10 <sup>-4</sup> | 0        | 1        | 0.20       | 1266.21   | 1.42       | 0.01823        | 35.33         | 0.644        | (7.067 ± 0.047) · 10 <sup>-2</sup>  | 0.014              | -                         | -                         |
| M_0W0.30         | 2·10 <sup>-4</sup> | 2·10 <sup>-4</sup> | 0        | 0.52     | 0.30       | 1304.95   | 2.16       | 0.01749        | 52.12         | 0.911        | (6.949 ± 0.072) · 10 <sup>-2</sup>  | 0.011              | -                         | -                         |
| M_0W0.40         | 2·10 <sup>-4</sup> | 2·10 <sup>-4</sup> | 0        | 0.36     | 0.40       | 1293.14   | 2.78       | 0.02089        | 72.06         | 1.505        | (7.21 ± 0.12) · 10 <sup>-2</sup>    | 0.0085             | -                         | -                         |
| M_0W0.50         | 2·10 <sup>-4</sup> | 2·10 <sup>-4</sup> | 0        | 0.24     | 0.50       | 1313.37   | 3.56       | 0.01908        | 86.91         | 1.658        | (6.95 ± 0.14) · 10 <sup>-2</sup>    | 0.0072             | -                         | -                         |
| M_0W0.60         | 2·10 <sup>-4</sup> | 2·10 <sup>-4</sup> | 0        | 0.175    | 0.60       | 1233.70   | 4.39       | 0.01845        | 102.5         | 1.890        | (6.83 ± 0.20) · 10 <sup>-2</sup>    | 0.0051             | -                         | -                         |
| M_0W0.80         | 2·10 <sup>-4</sup> | 2·10 <sup>-4</sup> | 0        | 0.118    | 0.80       | 1329.22   | 5.74       | 0.02050        | 139.9         | 2.861        | (6.98 ± 0.29) · 10 <sup>-2</sup>    | 0.0044             | -                         | -                         |
| M_0W1.00         | 2·10 <sup>-4</sup> | 2·10 <sup>-4</sup> | 0        | 0.087    | 1.00       | 1339.16   | 7.03       | 0.02186        | 178.5         | 3.901        | (7.14 ± 0.43) · 10 <sup>-2</sup>    | 0.0041             | -                         | -                         |
| M_0W1.50         | 2·10 <sup>-4</sup> | 2·10 <sup>-4</sup> | 0        | 0.048    | 1.50       | 1433.08   | 11.2       | 0.01528        | 253.7         | 3.890        | (6.77 ± 0.73) · 10 <sup>-2</sup>    | 0.0031             | -                         | -                         |
| M_0W2.00         | 2·10 <sup>-4</sup> | 2·10 <sup>-4</sup> | 0        | 0.031    | 2.00       | 1489.96   | 16.7       | 0.01550        | 304.5         | 4.713        | (6.09 ± 0.81) · 10 <sup>-2</sup>    | 0.0022             | -                         | -                         |
| M_2W0.10         | 2·10 <sup>-4</sup> | 2·10 <sup>-4</sup> | 2        | 2.0      | 0.10       | 1028.6    | 0.84       | 0.1666         | 14.82         | 2.469        | (5.927 ± 0.021) · 10 <sup>-2</sup>  | 0.11               | -                         | -                         |
| M_2W0.10         | 2·10 <sup>-4</sup> | 2·10 <sup>-4</sup> | 2        | 1.5      | 0.10       | 1114.23   | 1.03       | 0.1640         | 12.13         | 1.990        | (4.854 ± 0.020) · 10 <sup>-2</sup>  | 0.11               | -                         | -                         |
| M_2W0.20         | 2·10 <sup>-4</sup> | 2·10 <sup>-4</sup> | 2        | 1        | 0.20       | 1276.66   | 0.85       | 0.3822         | 59.07         | 22.57        | (11.81 ± 0.12) · 10 <sup>-2</sup>   | 0.29               | -                         | -                         |
| M_2W0.30         | 2·10 <sup>-4</sup> | 2·10 <sup>-4</sup> | 2        | 0.52     | 0.30       | 1237.98   | 1.08       | 0.6644         | 104.5         | 69.41        | (13.94 ± 0.29) · 10 <sup>-2</sup>   | 0.42               | -                         | -                         |
| M_2W0.40         | 2·10 <sup>-4</sup> | 2·10 <sup>-4</sup> | 2        | 0.36     | 0.40       | 1225.51   | 1.28       | 0.8895         | 157.0         | 139.6        | (15.70 ± 0.50) · 10 <sup>-2</sup>   | 0.50               | -                         | -                         |
| M_2W0.50         | 2·10 <sup>-4</sup> | 2·10 <sup>-4</sup> | 2        | 0.24     | 0.50       | 1250.13   | 1.65       | 1.030          | 190.1         | 195.7        | (15.21 ± 0.45) · 10 <sup>-2</sup>   | 0.54               | -                         | -                         |
| M_2W0.60         | 2·10 <sup>-4</sup> | 2·10 <sup>-4</sup> | 2        | 0.175    | 0.60       | 1178.19   | 1.93       | 1.105          | 233.5         | 257.7        | (15.57 ± 0.54) · 10 <sup>-2</sup>   | 0.52               | -                         | -                         |
| M_2W0.80         | 2·10 <sup>-4</sup> | 2·10 <sup>-4</sup> | 2        | 0.118    | 0.80       | 1252.24   | 2.36       | 1.247          | 339.3         | 422.9        | (16.96 ± 0.39) · 10 <sup>-2</sup>   | 0.57               | -                         | -                         |
| M_2W1.00         | 2·10 <sup>-4</sup> | 2·10 <sup>-4</sup> | 2        | 0.087    | 1.00       | 1261.90   | 3.03       | 1.424          | 413.3         | 588.4        | (16.53 ± 0.38) · 10 <sup>-2</sup>   | 0.57               | -                         | -                         |
| M_2W1.50         | 2·10 <sup>-4</sup> | 2·10 <sup>-4</sup> | 2        | 0.048    | 1.50       | 1285.2    | 4.52       | 1.983          | 625.0         | 1246         | (16.7 ± 1.2) · 10 <sup>-2</sup>     | 0.55               | -                         | -                         |
| M_2W2.00         | 2·10 <sup>-4</sup> | 2·10 <sup>-4</sup> | 2        | 0.031    | 2.00       | 1329.72   | 6.47       | 1.845          | 790.1         | 1450         | (15.8 ± 2.3) · 10 <sup>-2</sup>     | 0.44               | -                         | -                         |
| M_0W0.20_Pm0.25  | 2·10 <sup>-4</sup> | 8·10 <sup>-4</sup> | 0        | 1.0      | 0.20       | 1288.08   | 1.42       | 0.01828        | 35.1 (8.776)  | 0.6417       | (7.021 ± 0.044) · 10 <sup>-2</sup>  | 0.014              | -                         | -                         |
| M_0W0.20_Pm4     | 8·10 <sup>-4</sup> | 2·10 <sup>-4</sup> | 0        | 1.0      | 0.20       | 1305.14   | 1.62       | 0.00620        | 7.729 (30.92) | 0.04792      | (6.184 ± 0.049) · 10 <sup>-2</sup>  | 0.013              | -                         | -                         |
| M_2W0.20_Pm0.25  | 2·10 <sup>-4</sup> | 8·10 <sup>-4</sup> | 2        | 1.0      | 0.20       | 1241.23   | 0.85       | 0.3814         | 59.30 (14.80) | 22.39        | (11.840 ± 0.098) · 10 <sup>-2</sup> | 0.29               | -                         | -                         |
| M_2W0.20_Pm4     | 8·10 <sup>-4</sup> | 2·10 <sup>-4</sup> | 2        | 1.0      | 0.20       | 1295.54   | 1.30       | 0.3036         | 9.566 (38.27) | 29.04        | (7.653 ± 0.051) · 10 <sup>-2</sup>  | 0.23               | -                         | -                         |
| 512 <sup>3</sup> | $\nu$              | $\eta$             | $\Omega$ | $\phi_0$ | R          | $t_{tot}$ | $t_{turn}$ | $k_\omega/k_f$ | Re (Rm)       | Re $_\omega$ | $u_{rms}$                           | $u_{rot}/u_{tot}$  | $r(t_{turn}^{-1})$        | $r_\omega(t_{turn}^{-1})$ |
| M_0W0.20_512     | 2·10 <sup>-4</sup> | 2·10 <sup>-4</sup> | 0        | 1        | 0.20       | 47.34     | 1.47       | 0.00581        | 34.02         | 0.1975       | (6.803 ± 0.041) · 10 <sup>-2</sup>  | 0.012              | -                         | -                         |
| M_0W0.60_512     | 2·10 <sup>-4</sup> | 2·10 <sup>-4</sup> | 0        | 0.175    | 0.60       | 598.85    | 4.531      | 0.01148        | 99.41         | 1.141        | (6.627 ± 0.19) · 10 <sup>-2</sup>   | -                  | -                         | -                         |
| M_2W0.60_512     | 2·10 <sup>-4</sup> | 2·10 <sup>-4</sup> | 2        | 0.175    | 0.60       | 339.57    | 2.13       | 1.174          | 211.0         | 247.8        | (14.07 ± 0.22) · 10 <sup>-2</sup>   | -                  | -                         | -                         |
| 256 <sup>3</sup> | $\nu$              | $\eta$             | $\Omega$ | $\phi_0$ | $\Delta t$ | R         | $t_{turn}$ | $k_\omega/k_f$ | Re (Rm)       | Re $_\omega$ | $u_{rot}/u_{tot}$                   | $r(t_{turn}^{-1})$ | $r_\omega(t_{turn}^{-1})$ |                           |
| M_0              | 2·10 <sup>-4</sup> | 2·10 <sup>-4</sup> | 0        | 1        | 0.02       | 0.2       | 1.42       | 0.01820        | 35.3          | 0.64         | 0.014                               | -                  | -                         |                           |
| M_0s             | 2·10 <sup>-4</sup> | 2·10 <sup>-4</sup> | 0        | 1        | 1          | 0.2       | 4.32       | 0.00061        | 11.6          | 0.007        | -                                   | -                  | -                         |                           |
| M_0c             | 2·10 <sup>-4</sup> | 2·10 <sup>-4</sup> | 0        | 1        | $\delta t$ | 0.2       | 1.46       | 0.01609        | 34.3          | 0.55         | -                                   | -                  | -                         |                           |
| M_0low†          | 2·10 <sup>-5</sup> | 2·10 <sup>-5</sup> | 0        | 1        | 0.02       | 0.2       | 3.05       | 0.5913         | 163.8         | 97.03        | -                                   | -                  | -                         |                           |
| M_0low_F2†       | 2·10 <sup>-5</sup> | 2·10 <sup>-5</sup> | 0        | 2        | 0.02       | 0.2       | 1.03       | 1.4231         | 486.9         | 708.34       | -                                   | -                  | -                         |                           |
| M_0lowc          | 2·10 <sup>-5</sup> | 2·10 <sup>-5</sup> | 0        | 1        | $\delta t$ | 0.2       | 1.38       | 0.08582        | 362.6         | 31.12        | -                                   | -                  | -                         |                           |
| M_0highcF10      | 2·10 <sup>-2</sup> | 2·10 <sup>-2</sup> | 0        | 10       | $\delta t$ | 0.2       | 0.61       | 0.03443        | 0.81          | 0.028        | -                                   | -                  | -                         |                           |
| M_2              | 2·10 <sup>-4</sup> | 2·10 <sup>-4</sup> | 2        | 1        | 0.02       | 0.2       | 0.84       | 0.3809         | 59.2          | 22.55        | 0.292                               | -                  | -                         |                           |
| M_2c             | 2·10 <sup>-4</sup> | 2·10 <sup>-4</sup> | 2        | 1        | $\delta t$ | 0.2       | 0.85       | 0.38179        | 58.5          | 22.35        | -                                   | -                  | -                         |                           |
| M_2W0.5†         | 2·10 <sup>-4</sup> | 2·10 <sup>-4</sup> | 2        | 1        | $\delta t$ | 0.5       | 0.29       | 0.64222        | 171.7         | 110.24       | -                                   | -                  | -                         |                           |
| M_2low†          | 2·10 <sup>-5</sup> | 2·10 <sup>-5</sup> | 2        | 1        | 0.02       | 0.2       | 2.91       | 1.60296        | 171.8         | 276.5        | -                                   | -                  | -                         |                           |

Table 2: Baroclinic (i.e. non-isothermal) runs without shear. In every model we use  $B_0=10^{-6}$  as seed field, all the new runs have  $\Delta t=0.02$ , and all have  $c_{s0}^2=1$ .

| 256 <sup>3</sup> | $\nu$             | $\chi$            | $\eta$            | $\tau_{cool}$ | $\Omega$ | $\phi_0$ | R          | $t_{tot}$ | $t_{turn}$ | $k_\omega/k_f$ | Re (Rm)        | $Re_\omega$ | $u_{rms}$                         | $u_{rot}/u_{tot}$ | $r(t_{turn}^{-1})$ | $r_\omega(t_{turn}^{-1})$ |
|------------------|-------------------|-------------------|-------------------|---------------|----------|----------|------------|-----------|------------|----------------|----------------|-------------|-----------------------------------|-------------------|--------------------|---------------------------|
| MB_0W0.20_notau  | $2 \cdot 10^{-4}$ | $2 \cdot 10^{-4}$ | $2 \cdot 10^{-4}$ | 0.1           | 0        | 2        | 0.20       | 1015.53   | 2.25       | 0.0304         | 22.23          | 0.675       | $(4.445 \pm 0.037) \cdot 10^{-2}$ | 0.015             | -                  | -                         |
| MB_0W0.20        | $2 \cdot 10^{-4}$ | $2 \cdot 10^{-4}$ | $2 \cdot 10^{-4}$ | -             | 0        | 1        | 0.20       | 905.98    | 2.69       | 0.1550         | 18.60          | 2.883       | $(3.720 \pm 0.038) \cdot 10^{-2}$ | 0.036             | -                  | -                         |
| MB_0W0.30_notau  | $2 \cdot 10^{-4}$ | $2 \cdot 10^{-4}$ | $2 \cdot 10^{-4}$ | 0.1           | 0        | 1.04     | 0.30       | 970.32    | 2.52       | 0.0101         | 44.69          | 0.451       | $(5.959 \pm 0.067) \cdot 10^{-2}$ | 0.011             | -                  | -                         |
| MB_0W0.30        | $2 \cdot 10^{-4}$ | $2 \cdot 10^{-4}$ | $2 \cdot 10^{-4}$ | -             | 0        | 0.52     | 0.30       | 1079.47   | 3.77       | 0.1748         | 29.84          | 5.215       | $(3.979 \pm 0.062) \cdot 10^{-2}$ | 0.040             | -                  | -                         |
| MB_0W0.40_notau  | $2 \cdot 10^{-4}$ | $2 \cdot 10^{-4}$ | $2 \cdot 10^{-4}$ | 0.1           | 0        | 0.72     | 0.40       | 964.04    | 3.23       | 0.0137         | 61.88          | 0.847       | $(6.19 \pm 0.10) \cdot 10^{-2}$   | 0.0076            | -                  | -                         |
| MB_0W0.40        | $2 \cdot 10^{-4}$ | $2 \cdot 10^{-4}$ | $2 \cdot 10^{-4}$ | -             | 0        | 0.36     | 0.40       | 1183.27   | 5.04       | 0.1744         | 39.77          | 6.930       | $(3.98 \pm 0.14) \cdot 10^{-2}$   | 0.037             | -                  | -                         |
| MB_0W0.50_notau  | $2 \cdot 10^{-4}$ | $2 \cdot 10^{-4}$ | $2 \cdot 10^{-4}$ | 0.1           | 0        | 0.48     | 0.50       | 980.79    | 4.19       | 0.0142         | 74.68          | 1.060       | $(5.97 \pm 0.14) \cdot 10^{-2}$   | 0.0072            | -                  | -                         |
| MB_0W0.50        | $2 \cdot 10^{-4}$ | $2 \cdot 10^{-4}$ | $2 \cdot 10^{-4}$ | -             | 0        | 0.24     | 0.50       | 1234.23   | 6.45       | 0.1655         | 48.50          | 8.018       | $(3.88 \pm 0.13) \cdot 10^{-2}$   | 0.030             | -                  | -                         |
| MB_0W0.60_notau  | $2 \cdot 10^{-4}$ | $2 \cdot 10^{-4}$ | $2 \cdot 10^{-4}$ | 0.1           | 0        | 0.35     | 0.60       | 998.6     | 5.14       | 0.0142         | 87.66          | 1.248       | $(5.84 \pm 0.16) \cdot 10^{-2}$   | 0.0065            | -                  | -                         |
| MB_0W0.60        | $2 \cdot 10^{-4}$ | $2 \cdot 10^{-4}$ | $2 \cdot 10^{-4}$ | -             | 0        | 0.175    | 0.60       | 1251.19   | 7.53       | 0.1633         | 59.99          | 9.777       | $(4.00 \pm 0.17) \cdot 10^{-2}$   | 0.024             | -                  | -                         |
| MB_0W0.80_notau  | $2 \cdot 10^{-4}$ | $2 \cdot 10^{-4}$ | $2 \cdot 10^{-4}$ | 0.1           | 0        | 0.236    | 0.80       | 1009.31   | 6.73       | 0.0183         | 191.1          | 2.174       | $(5.95 \pm 0.25) \cdot 10^{-2}$   | 0.0050            | -                  | -                         |
| MB_0W0.80        | $2 \cdot 10^{-4}$ | $2 \cdot 10^{-4}$ | $2 \cdot 10^{-4}$ | -             | 0        | 0.118    | 0.80       | 1252.50   | 8.69       | 0.1732         | 92.52          | 15.95       | $(4.63 \pm 0.31) \cdot 10^{-2}$   | 0.022             | -                  | -                         |
| MB_0W1.00_notau  | $2 \cdot 10^{-4}$ | $2 \cdot 10^{-4}$ | $2 \cdot 10^{-4}$ | 0.1           | 0        | 0.174    | 1.00       | 1020.70   | 8.32       | 0.0216         | 150.6          | 3.247       | $(6.03 \pm 0.33) \cdot 10^{-2}$   | 0.0040            | -                  | -                         |
| MB_0W1.00        | $2 \cdot 10^{-4}$ | $2 \cdot 10^{-4}$ | $2 \cdot 10^{-4}$ | -             | 0        | 0.087    | 1.00       | 1248.69   | 9.80       | 0.1828         | 128.6          | 23.31       | $(5.14 \pm 0.47) \cdot 10^{-2}$   | 0.022             | -                  | -                         |
| MB_0W1.50_notau  | $2 \cdot 10^{-4}$ | $2 \cdot 10^{-4}$ | $2 \cdot 10^{-4}$ | 0.1           | 0        | 0.096    | 1.50       | 1077.97   | 12.4       | 0.0168         | 229.5          | 3.852       | $(6.12 \pm 0.65) \cdot 10^{-2}$   | 0.0029            | -                  | -                         |
| MB_0W1.50        | $2 \cdot 10^{-4}$ | $2 \cdot 10^{-4}$ | $2 \cdot 10^{-4}$ | -             | 0        | 0.048    | 1.50       | 1248.71   | 13.4       | 0.2479         | 214.2          | 51.83       | $(5.71 \pm 0.87) \cdot 10^{-2}$   | 0.027             | -                  | -                         |
| MB_0W2.00_notau  | $2 \cdot 10^{-4}$ | $2 \cdot 10^{-4}$ | $2 \cdot 10^{-4}$ | 0.1           | 0        | 0.062    | 2.00       | 1164.33   | 18.8       | 0.0146         | 272.3          | 4.028       | $(5.45 \pm 0.85) \cdot 10^{-2}$   | 0.0016            | -                  | -                         |
| MB_0W2.00        | $2 \cdot 10^{-4}$ | $2 \cdot 10^{-4}$ | $2 \cdot 10^{-4}$ | -             | 0        | 0.031    | 2.00       | 1259.42   | 19.0       | 0.2886         | 273.4          | 75.96       | $(5.5 \pm 1.1) \cdot 10^{-2}$     | 0.020             | -                  | -                         |
| MB_0W0.60_tau001 | $2 \cdot 10^{-4}$ | $2 \cdot 10^{-4}$ | $2 \cdot 10^{-4}$ | 0.01          | 0        | 0.175    | 0.60       | crashed   | -          | -              | -              | -           | -                                 | -                 | -                  | -                         |
| MB_0W0.60_tau002 | $2 \cdot 10^{-4}$ | $2 \cdot 10^{-4}$ | $2 \cdot 10^{-4}$ | 0.02          | 0        | 0.175    | 0.60       | crashed   | -          | -              | -              | -           | -                                 | -                 | -                  | -                         |
| MB_0W0.60_tau005 | $2 \cdot 10^{-4}$ | $2 \cdot 10^{-4}$ | $2 \cdot 10^{-4}$ | 0.05          | 0        | 0.175    | 0.60       | 1224.46   | 5.71       | 0.1240         | 78.95          | 9.772       | $(5.26 \pm 0.22) \cdot 10^{-2}$   | 0.016             | -                  | -                         |
| MB_0W0.60_tau    | $2 \cdot 10^{-4}$ | $2 \cdot 10^{-4}$ | $2 \cdot 10^{-4}$ | 0.1           | 0        | 0.175    | 0.60       | 1251.19   | 7.52       | 0.1633         | 59.99          | 9.777       | $(3.99 \pm 0.17) \cdot 10^{-2}$   | 0.024             | -                  | -                         |
| MB_0W0.60_tau02  | $2 \cdot 10^{-4}$ | $2 \cdot 10^{-4}$ | $2 \cdot 10^{-4}$ | 0.2           | 0        | 0.175    | 0.60       | 1264.19   | 9.56       | 0.1958         | 47.19          | 9.223       | $(3.14 \pm 0.13) \cdot 10^{-2}$   | 0.038             | -                  | -                         |
| MB_0W0.60_tau05  | $2 \cdot 10^{-4}$ | $2 \cdot 10^{-4}$ | $2 \cdot 10^{-4}$ | 0.5           | 0        | 0.175    | 0.60       | 1264.94   | 10.38      | 0.1919         | 43.42          | 8.324       | $(2.89 \pm 0.10) \cdot 10^{-2}$   | 0.039             | -                  | -                         |
| MB_0W0.60_tau1   | $2 \cdot 10^{-4}$ | $2 \cdot 10^{-4}$ | $2 \cdot 10^{-4}$ | 1.0           | 0        | 0.175    | 0.60       | 1248.29   | 8.80       | 0.1520         | 51.21          | 7.774       | $(3.41 \pm 0.11) \cdot 10^{-2}$   | 0.026             | -                  | -                         |
| MB_2W0.20        | $2 \cdot 10^{-4}$ | $2 \cdot 10^{-4}$ | $2 \cdot 10^{-4}$ | 0.1           | 2        | 2        | 0.20       | 891.15    | 2.10       | 0.4497         | 23.82          | 10.71       | $(4.764 \pm 0.035) \cdot 10^{-2}$ | 0.42              | -                  | -                         |
| MB_2W0.30        | $2 \cdot 10^{-4}$ | $2 \cdot 10^{-4}$ | $2 \cdot 10^{-4}$ | 0.1           | 2        | 1.04     | 0.30       | 1062.24   | 2.62       | 0.5963         | 42.92          | 25.59       | $(5.722 \pm 0.060) \cdot 10^{-2}$ | 0.54              | -                  | -                         |
| MB_2W0.40        | $2 \cdot 10^{-4}$ | $2 \cdot 10^{-4}$ | $2 \cdot 10^{-4}$ | 0.1           | 2        | 0.72     | 0.40       | 1108.78   | 2.82       | 0.6709         | 70.95          | 47.59       | $(7.095 \pm 0.11) \cdot 10^{-2}$  | 0.60              | -                  | -                         |
| MB_2W0.50        | $2 \cdot 10^{-4}$ | $2 \cdot 10^{-4}$ | $2 \cdot 10^{-4}$ | 0.1           | 2        | 0.48     | 0.50       | 1176.45   | 3.95       | 0.6898         | 79.28          | 54.66       | $(6.342 \pm 0.26) \cdot 10^{-2}$  | 0.60              | -                  | -                         |
| MB_2W0.60        | $2 \cdot 10^{-4}$ | $2 \cdot 10^{-4}$ | $2 \cdot 10^{-4}$ | 0.1           | 2        | 0.35     | 0.60       | 1190.03   | 4.70       | 0.6984         | 95.95          | 66.99       | $(6.397 \pm 0.20) \cdot 10^{-2}$  | 0.62              | -                  | -                         |
| MB_2W0.80        | $2 \cdot 10^{-4}$ | $2 \cdot 10^{-4}$ | $2 \cdot 10^{-4}$ | 0.1           | 2        | 0.236    | 0.80       | 1174.07   | 5.33       | 0.7139         | 150.8          | 107.5       | $(7.541 \pm 0.49) \cdot 10^{-2}$  | 0.57              | -                  | -                         |
| MB_2W1.00        | $2 \cdot 10^{-4}$ | $2 \cdot 10^{-4}$ | $2 \cdot 10^{-4}$ | 0.1           | 2        | 0.174    | 1.00       | 1160.27   | 5.65       | 0.7419         | 222.8          | 165.0       | $(8.912 \pm 0.77) \cdot 10^{-2}$  | 0.60              | -                  | -                         |
| MB_2W1.50        | $2 \cdot 10^{-4}$ | $2 \cdot 10^{-4}$ | $2 \cdot 10^{-4}$ | 0.1           | 2        | 0.096    | 1.50       | 1175.55   | 8.33       | 0.8140         | 343.3          | 278.5       | $(9.154 \pm 1.2) \cdot 10^{-2}$   | 0.54              | -                  | -                         |
| MB_2W2.00        | $2 \cdot 10^{-4}$ | $2 \cdot 10^{-4}$ | $2 \cdot 10^{-4}$ | 0.1           | 2        | 0.062    | 2.00       | 1194.15   | 12.6       | 0.8870         | 407.1          | 358.3       | $(8.142 \pm 1.2) \cdot 10^{-2}$   | 0.43              | -                  | -                         |
| MB_0W_Pm0.25     | $2 \cdot 10^{-4}$ | $8 \cdot 10^{-4}$ | $2 \cdot 10^{-4}$ | 0.01          | 0        | 2.00     | 0.20       | 1129.75   | 1.29       | 0.0762         | 38.78 (9.694)  | 2.954       | $(7.755 \pm 0.074) \cdot 10^{-2}$ | 0.019             | -                  | -                         |
| MB_0W_Pm4        | $8 \cdot 10^{-4}$ | $2 \cdot 10^{-4}$ | $2 \cdot 10^{-4}$ | 0.01          | 0        | 2.00     | 0.20       | 1154.10   | 2.77       | 0.0770         | 4.499 (18.00)  | 0.346       | $(3.600 \pm 0.035) \cdot 10^{-2}$ | 0.022             | -                  | -                         |
| MB_2W_Pm0.25     | $2 \cdot 10^{-4}$ | $8 \cdot 10^{-4}$ | $2 \cdot 10^{-4}$ | 0.01          | 2        | 2.00     | 0.20       | 1138.86   | 2.11       | 0.450          | 23.65 (5.914)  | 10.65       | $(4.731 \pm 0.033) \cdot 10^{-2}$ | 0.42              | -                  | -                         |
| MB_2W_Pm4        | $8 \cdot 10^{-4}$ | $2 \cdot 10^{-4}$ | $2 \cdot 10^{-4}$ | 0.01          | 2        | 2.00     | 0.20       | 1158.22   | 2.16       | 0.419          | 11.59 (23.17)  | 4.858       | $(4.635 \pm 0.035) \cdot 10^{-2}$ | 0.39              | -                  | -                         |
| 512 <sup>3</sup> | $\nu$             | $\chi$            | $\eta$            | $\tau_{cool}$ | $\Omega$ | $\phi_0$ | R          | $t_{tot}$ | $t_{turn}$ | $k_\omega/k_f$ | Re (Rm)        | $Re_\omega$ | $u_{rms}$                         | $u_{rot}/u_{tot}$ | $r(t_{turn}^{-1})$ | $r_\omega(t_{turn}^{-1})$ |
| MB_0W0.20_512    | $2 \cdot 10^{-4}$ | $2 \cdot 10^{-4}$ | $2 \cdot 10^{-4}$ | -             | 0        | 1        | 0.2        | 44.10     | 1.69       | 0.00717        | 29.6           | 0.21        | $(5.884 \pm 0.072) \cdot 10^{-2}$ | -                 | -                  | -                         |
| MB_0W0.60_512    | $2 \cdot 10^{-4}$ | $2 \cdot 10^{-4}$ | $2 \cdot 10^{-4}$ | 0.1           | 0        | 0.35     | 0.60       | 199.97    | 7.10       | 0.09355        | 63.5           | 5.92        | $(4.23 \pm 0.20) \cdot 10^{-2}$   | -                 | -                  | -                         |
| MB_2W0.60_512    | $2 \cdot 10^{-4}$ | $2 \cdot 10^{-4}$ | $2 \cdot 10^{-4}$ | 0.1           | 2        | 0.35     | 0.60       | 199.18    | 4.69       | 0.7196         | 96.1           | 69.1        | $(6.40 \pm 0.26) \cdot 10^{-2}$   | -                 | -                  | -                         |
| 256 <sup>3</sup> | $\nu$             | $\chi$            | $\eta$            | $\tau_{cool}$ | $\Omega$ | $\phi_0$ | $\Delta t$ | R         | $t_{tot}$  | $t_{turn}$     | $k_\omega/k_f$ | Re (Rm)     | $Re_\omega$                       | $u_{rot}/u_{tot}$ | $r(t_{turn}^{-1})$ | $r_\omega(t_{turn}^{-1})$ |
| MB_0             | $2 \cdot 10^{-4}$ | $2 \cdot 10^{-4}$ | $2 \cdot 10^{-4}$ | -             | 0        | 1        | 0.02       | 0.2       | -          | 1.65           | 0.0878         | 30.3        | 0.27                              | -                 | -                  | -                         |
| MB_0c            | $2 \cdot 10^{-4}$ | $2 \cdot 10^{-4}$ | $2 \cdot 10^{-4}$ | -             | 0        | 1        | $\delta t$ | 0.2       | -          | 1.65           | 0.00876        | 30.3        | 0.27                              | -                 | -                  | -                         |
| MB_0highcF10     | $2 \cdot 10^{-2}$ | $2 \cdot 10^{-4}$ | $2 \cdot 10^{-2}$ | -             | 0        | 10       | $\delta t$ | 0.2       | -          | 0.64           | 0.01376        | 0.78        | 0.0108                            | -                 | -                  | -                         |
| MB_0lowc         | $5 \cdot 10^{-5}$ | $2 \cdot 10^{-4}$ | $5 \cdot 10^{-5}$ | -             | 0        | 1        | $\delta t$ | 0.2       | -          | 1.61           | 0.02876        | 124.1       | 3.57                              | -                 | -                  | -                         |
| MB_0low          | $5 \cdot 10^{-5}$ | $2 \cdot 10^{-4}$ | $5 \cdot 10^{-5}$ | -             | 0        | 1        | 0.02       | 0.2       | -          | 1.61           | 0.03046        | 124.4       | 3.79                              | -                 | -                  | -                         |
| MB_0low2c        | $2 \cdot 10^{-5}$ | $2 \cdot 10^{-4}$ | $2 \cdot 10^{-5}$ | -             | 0        | 1        | $\delta t$ | 0.2       | -          | 1.60           | 0.0434         | 313.1       | 13.58                             | -                 | -                  | -                         |
| MB_2             | $2 \cdot 10^{-4}$ | $2 \cdot 10^{-4}$ | $2 \cdot 10^{-4}$ | -             | 2        | 1        | 0.02       | 0.2       | -          | 1.08           | 0.340          | 46.5        | 15.83                             | -                 | -                  | -                         |
| MB_2c            | $2 \cdot 10^{-4}$ | $2 \cdot 10^{-4}$ | $2 \cdot 10^{-4}$ | -             | 2        | 1        | $\delta t$ | 0.2       | -          | 1.06           | 0.343          | 47.0        | 16.12                             | -                 | -                  | -                         |
| MB_2low†         | $2 \cdot 10^{-5}$ | $2 \cdot 10^{-4}$ | $2 \cdot 10^{-5}$ | -             | 2        | 1        | 0.02       | 0.2       | -          | 0.96           | 0.6172         | 522.2       | 323.0                             | -                 | -                  | -                         |
| MB_0W0.1         | $2 \cdot 10^{-2}$ | $2 \cdot 10^{-2}$ | $2 \cdot 10^{-2}$ | -             | 0        | 1        | 0.02       | 0.1       | -          | 15.31          | 0.00076        | 0.0082      | 0.00001                           | -                 | -                  | -                         |
| MB_0W0.2         | $2 \cdot 10^{-2}$ | $2 \cdot 10^{-2}$ | $2 \cdot 10^{-2}$ | -             | 0        | 1        | 0.02       | 0.2       | -          | 7.84           | 0.00419        | 0.0638      | 0.00027                           | -                 | -                  | -                         |
| MB_0W0.5         | $2 \cdot 10^{-2}$ | $2 \cdot 10^{-2}$ | $2 \cdot 10^{-2}$ | -             | 0        | 1        | 0.02       | 0.5       | -          | 1.36           | 0.01923        | 0.9209      | 0.01772                           | -                 | -                  | -                         |
| MB_0W1           | $2 \cdot 10^{-2}$ | $2 \cdot 10^{-2}$ | $2 \cdot 10^{-2}$ | -             | 0        | 1        | 0.02       | 1.0       | -          | 0.46           | 0.06042        | 5.399       | 0.3263                            | -                 | -                  | -                         |

Table 3: Models with sinusoidal shearing velocity profile. In every model we use  $B_0=10^{-6}$  as seed field,  $\Delta t=0.02$  as interval between two different explosions, and an amplitude of the shearing profile  $A=0.2$ . ND stands for the growth rates not determined, even though dynamo was present.

| 256 <sup>3</sup>   | $\nu$               | $\chi$            | $\eta$                | $\tau_{cool}$ | $A$  | $\phi_0$ | R    | $t_{tot}$ | $t_{turn}$ | $k_w/k_f$ | Re(Rm)      | Re $_{\omega}$ | $u_{rot,0}/u_{tot}$ | $u_{rot}/u_{tot}$ | $r(t_{turn}^{-1})$    | $r_{\omega}(t_{turn}^{-1})$ |
|--------------------|---------------------|-------------------|-----------------------|---------------|------|----------|------|-----------|------------|-----------|-------------|----------------|---------------------|-------------------|-----------------------|-----------------------------|
| M_S_Pm0.1          | $2 \cdot 10^{-4}$   | -                 | $20 \cdot 10^{-4}$    | -             | 0.20 | 1        | 0.2  | 4189.19   | 0.637      | 0.0915    | 78.5 (7.85) | 7.849          | 0.819               | 0.899             | -                     | $1.052 \cdot 10^{-2}$       |
| M_S_Pm0.25         | $2 \cdot 10^{-4}$   | -                 | $8 \cdot 10^{-4}$     | -             | 0.20 | 1        | 0.2  | 2277.66   | 0.635      | 0.0919    | 78.8 (19.7) | 19.70          | 0.811               | 0.894             | $3.261 \cdot 10^{-3}$ | $8.573 \cdot 10^{-3}$       |
| M_S_Pm0.5          | $2 \cdot 10^{-4}$   | -                 | $4 \cdot 10^{-4}$     | -             | 0.20 | 1        | 0.2  | 3492.59   | 0.634      | 0.0912    | 78.9 (39.5) | 39.46          | 0.810               | 0.873             | $1.224 \cdot 10^{-2}$ | $9.333 \cdot 10^{-3}$       |
| M_S_Pm0.75         | $2 \cdot 10^{-4}$   | -                 | $2.667 \cdot 10^{-4}$ | -             | 0.20 | 1        | 0.2  | 3927.51   | 0.634      | 0.0911    | 78.9 (59.2) | 59.20          | 0.809               | 0.867             | $2.254 \cdot 10^{-2}$ | $1.096 \cdot 10^{-2}$       |
| M_S_Pm1            | $2 \cdot 10^{-4}$   | -                 | $2 \cdot 10^{-4}$     | -             | 0.20 | 1        | 0.2  | 3559.77   | 0.633      | 0.0910    | 78.9 (78.9) | 78.94          | 0.806               | 0.861             | $2.783 \cdot 10^{-2}$ | $1.022 \cdot 10^{-2}$       |
| M_S_Pm1.25         | $2.5 \cdot 10^{-4}$ | -                 | $2 \cdot 10^{-4}$     | -             | 0.20 | 1        | 0.2  | 3965.97   | 0.636      | 0.0910    | 62.9 (78.6) | 78.64          | 0.825               | 0.852             | $2.861 \cdot 10^{-2}$ | $9.176 \cdot 10^{-3}$       |
| M_S_Pm1.5          | $3 \cdot 10^{-4}$   | -                 | $2 \cdot 10^{-4}$     | -             | 0.20 | 1        | 0.2  | 3811.68   | 0.637      | 0.0910    | 52.3 (78.5) | 78.50          | 0.817               | 0.865             | $3.073 \cdot 10^{-2}$ | $1.001 \cdot 10^{-2}$       |
| M_S_Pm2            | $4 \cdot 10^{-4}$   | -                 | $2 \cdot 10^{-4}$     | -             | 0.20 | 1        | 0.2  | 4765.49   | 0.640      | 0.0914    | 39.0 (78.1) | 78.07          | 0.824               | 0.872             | $3.438 \cdot 10^{-2}$ | $9.378 \cdot 10^{-3}$       |
| M_S_Pm4            | $8 \cdot 10^{-4}$   | -                 | $2 \cdot 10^{-4}$     | -             | 0.20 | 1        | 0.2  | 4757.68   | 0.649      | 0.0922    | 19.3 (77.0) | 76.99          | 0.848               | -                 | -                     | -                           |
| M_S_Pm10           | $20 \cdot 10^{-4}$  | -                 | $2 \cdot 10^{-4}$     | -             | 0.20 | 1        | 0.2  | 3340.23   | 0.672      | 0.0947    | 7.44 (74.4) | 74.43          | 0.903               | -                 | -                     | -                           |
| M_S_W0.10          | $2 \cdot 10^{-4}$   | -                 | $2 \cdot 10^{-4}$     | -             | 0.20 | 2        | 0.10 | 3012.18   | 0.33       | 0.04733   | 37.5        | 1.775          | 0.888               | -                 | -                     | -                           |
| M_S_W0.20          | $2 \cdot 10^{-4}$   | -                 | $2 \cdot 10^{-4}$     | -             | 0.20 | 1        | 0.20 | 3332.61   | 0.63       | 0.09071   | 78.8        | 7.103          | 0.809               | 0.855             | $2.616 \cdot 10^{-2}$ | $1.022 \cdot 10^{-2}$       |
| M_S_W0.30          | $2 \cdot 10^{-4}$   | -                 | $2 \cdot 10^{-4}$     | -             | 0.20 | 0.52     | 0.30 | 4923.52   | 0.95       | 0.1372    | 118.2       | 15.98          | 0.818               | 0.861             | $3.997 \cdot 10^{-2}$ | $1.233 \cdot 10^{-2}$       |
| M_S_W0.40          | $2 \cdot 10^{-4}$   | -                 | $2 \cdot 10^{-4}$     | -             | 0.20 | 0.36     | 0.40 | 4867.96   | 1.26       | 0.1819    | 159.0       | 28.42          | 0.807               | 0.851             | $5.017 \cdot 10^{-2}$ | $2.273 \cdot 10^{-2}$       |
| M_S_W0.50          | $2 \cdot 10^{-4}$   | -                 | $2 \cdot 10^{-4}$     | -             | 0.20 | 0.24     | 0.50 | 4889.66   | 1.58       | 0.2275    | 197.5       | 44.37          | 0.818               | 0.861             | $7.514 \cdot 10^{-2}$ | $2.572 \cdot 10^{-2}$       |
| M_S_W0.60          | $2 \cdot 10^{-4}$   | -                 | $2 \cdot 10^{-4}$     | -             | 0.20 | 0.175    | 0.60 | 4092.11   | 1.90       | 0.2738    | 236.5       | 63.89          | 0.812               | 0.862             | $8.791 \cdot 10^{-2}$ | $3.361 \cdot 10^{-2}$       |
| M_S_W0.80          | $2 \cdot 10^{-4}$   | -                 | $2 \cdot 10^{-4}$     | -             | 0.20 | 0.118    | 0.80 | 4908.57   | 2.51       | 0.3607    | 319.3       | 113.5          | 0.812               | 0.846             | $1.190 \cdot 10^{-1}$ | $4.175 \cdot 10^{-2}$       |
| M_S_W1.00          | $2 \cdot 10^{-4}$   | -                 | $2 \cdot 10^{-4}$     | -             | 0.20 | 0.087    | 1.00 | 4918.58   | 3.08       | 0.4455    | 404.7       | 177.5          | 0.805               | 0.847             | $1.444 \cdot 10^{-1}$ | $5.803 \cdot 10^{-2}$       |
| M_S_W1.50          | $2 \cdot 10^{-4}$   | -                 | $2 \cdot 10^{-4}$     | -             | 0.20 | 0.048    | 1.50 | 1217.34   | 4.85       | 0.6884    | 579.9       | 399.1          | 0.804               | 0.840             | $1.729 \cdot 10^{-1}$ | $5.959 \cdot 10^{-2}$       |
| M_S_W2.00          | $2 \cdot 10^{-4}$   | -                 | $2 \cdot 10^{-4}$     | -             | 0.20 | 0.031    | 2.00 | 1333.81   | 3.48       | 0.4909    | 359.4       | 176.4          | 0.942               | -                 | $1.476 \cdot 10^{-1}$ | $5.058 \cdot 10^{-2}$       |
| MB_S_W0.20         | $2 \cdot 10^{-4}$   | $2 \cdot 10^{-4}$ | $2 \cdot 10^{-4}$     | 0.1           | 0.20 | 2        | 0.20 | 1710.04   | 0.68       | 0.1102    | 73.00       | 8.046          | 0.97                | 0.97              | $2.433 \cdot 10^{-2}$ | $8.832 \cdot 10^{-3}$       |
| MB_S_W0.30         | $2 \cdot 10^{-4}$   | $2 \cdot 10^{-4}$ | $2 \cdot 10^{-4}$     | 0.1           | 0.20 | 1.04     | 0.30 | 2307.15   | 1.02       | 0.1628    | 110.2       | 17.82          | 0.96                | 0.96              | $3.377 \cdot 10^{-2}$ | $1.116 \cdot 10^{-2}$       |
| MB_S_W0.40         | $2 \cdot 10^{-4}$   | $2 \cdot 10^{-4}$ | $2 \cdot 10^{-4}$     | 0.1           | 0.20 | 0.72     | 0.40 | 2401.10   | 1.35       | 0.2165    | 148.7       | 32.19          | 0.95                | 0.93              | $3.942 \cdot 10^{-2}$ | $1.556 \cdot 10^{-2}$       |
| MB_S_W0.50         | $2 \cdot 10^{-4}$   | $2 \cdot 10^{-4}$ | $2 \cdot 10^{-4}$     | 0.1           | 0.20 | 0.48     | 0.50 | 2444.66   | 1.68       | 0.2590    | 185.9       | 48.15          | 0.95                | 0.92              | $5.656 \cdot 10^{-2}$ | $2.470 \cdot 10^{-2}$       |
| MB_S_W0.60         | $2 \cdot 10^{-4}$   | $2 \cdot 10^{-4}$ | $2 \cdot 10^{-4}$     | 0.1           | 0.20 | 0.35     | 0.60 | 2448.34   | 2.02       | 0.3010    | 223.3       | 67.21          | 0.96                | 0.93              | $6.921 \cdot 10^{-2}$ | $2.768 \cdot 10^{-2}$       |
| MB_S_W0.80         | $2 \cdot 10^{-4}$   | $2 \cdot 10^{-4}$ | $2 \cdot 10^{-4}$     | 0.1           | 0.20 | 0.236    | 0.80 | 2407.49   | 2.64       | 0.3889    | 302.9       | 117.8          | 0.94                | 0.92              | $9.382 \cdot 10^{-2}$ | $4.174 \cdot 10^{-2}$       |
| MB_S_W1.00         | $2 \cdot 10^{-4}$   | $2 \cdot 10^{-4}$ | $2 \cdot 10^{-4}$     | 0.1           | 0.20 | 0.174    | 1.00 | 2342.14   | 3.25       | 0.4744    | 384.4       | 182.3          | 0.93                | 0.91              | $1.202 \cdot 10^{-1}$ | $6.614 \cdot 10^{-2}$       |
| MB_S_W1.50         | $2 \cdot 10^{-4}$   | $2 \cdot 10^{-4}$ | $2 \cdot 10^{-4}$     | 0.1           | 0.20 | 0.096    | 1.50 | 2421.20   | 4.80       | 0.6864    | 586.3       | 402.2          | 0.92                | 0.88              | $1.516 \cdot 10^{-1}$ | $8.403 \cdot 10^{-2}$       |
| MB_S_W2.00         | $2 \cdot 10^{-4}$   | $2 \cdot 10^{-4}$ | $2 \cdot 10^{-4}$     | 0.1           | 0.20 | 0.062    | 2.00 | 2421.66   | 6.44       | 0.9191    | 777.1       | 713.7          | 0.95                | 0.87              | $2.245 \cdot 10^{-1}$ | $1.137 \cdot 10^{-1}$       |
| MB_S_W0.50_tau0005 | $2 \cdot 10^{-4}$   | $2 \cdot 10^{-4}$ | $2 \cdot 10^{-4}$     | 0.005         | 0.20 | 0.48     | 0.50 | 1245.53   | 1.58       | 0.2232    | 198.4       | 44.28          | 0.81                | 0.77              | $5.863 \cdot 10^{-2}$ | $3.137 \cdot 10^{-2}$       |
| MB_S_W0.50_tau001  | $2 \cdot 10^{-4}$   | $2 \cdot 10^{-4}$ | $2 \cdot 10^{-4}$     | 0.01          | 0.20 | 0.48     | 0.50 | 1277.6    | 1.59       | 0.2258    | 196.1       | 44.27          | 0.84                | 0.80              | $5.993 \cdot 10^{-2}$ | $2.776 \cdot 10^{-2}$       |
| MB_S_W0.50_tau05   | $2 \cdot 10^{-4}$   | $2 \cdot 10^{-4}$ | $2 \cdot 10^{-4}$     | 0.05          | 0.20 | 0.48     | 0.50 | 1297.98   | 1.68       | 0.2362    | 187.5       | 44.28          | 0.92                | 0.88              | $7.864 \cdot 10^{-2}$ | $3.164 \cdot 10^{-2}$       |
| MB_S_W0.50_tau01   | $2 \cdot 10^{-4}$   | $2 \cdot 10^{-4}$ | $2 \cdot 10^{-4}$     | 0.1           | 0.20 | 0.48     | 0.50 | 1297.98   | 1.70       | 0.2410    | 183.7       | 44.28          | 0.95                | 0.93              | $6.769 \cdot 10^{-2}$ | $3.251 \cdot 10^{-2}$       |
| MB_S_W0.50_notau   | $2 \cdot 10^{-4}$   | $2 \cdot 10^{-4}$ | $2 \cdot 10^{-4}$     | -             | 0.20 | 0.48     | 0.50 | 979.59    | 1.57       | 0.2225    | 199.0       | 44.29          | 0.79                | 0.81              | $7.601 \cdot 10^{-2}$ | $3.203 \cdot 10^{-2}$       |
| MB_S_W0.20_notau   | $2 \cdot 10^{-4}$   | $2 \cdot 10^{-4}$ | $2 \cdot 10^{-4}$     | -             | 0.20 | 1        | 0.20 | 1769.62   | 0.65       | 0.0925    | 76.75       | 7.100          | 0.85                | 0.87              | $3.255 \cdot 10^{-2}$ | $9.601 \cdot 10^{-3}$       |
| 512 <sup>3</sup>   | $\nu$               | $\chi$            | $\eta$                | $\tau_{cool}$ | $A$  | $\phi_0$ | R    | $t_{tot}$ | $t_{turn}$ | $k_w/k_f$ | Re(Rm)      | Re $_{\omega}$ | $u_{rot,0}/u_{tot}$ | $u_{rot}/u_{tot}$ | $r(t_{turn}^{-1})$    | $r_{\omega}(t_{turn}^{-1})$ |
| M_0A020_512        | $2 \cdot 10^{-4}$   | -                 | $2 \cdot 10^{-4}$     | -             | 0.20 | 1        | 0.2  | 1606.63   | 0.64       | 0.091     | 78.5        | 7.10           | 0.83                | -                 | 0.0264                | 0.0107                      |
| M_0A020_512        | $1 \cdot 10^{-4}$   | -                 | $1 \cdot 10^{-4}$     | -             | 0.20 | 1        | 0.2  | 1950.99   | 0.64       | 0.090     | 157.0       | 14.2           | -                   | -                 | 0.0348                | 0.0162                      |
| M_0A060_512        | $2 \cdot 10^{-4}$   | -                 | $2 \cdot 10^{-4}$     | -             | 0.60 | 1        | 0.2  | 1642.89   | 1.98       | 0.281     | 227.3       | 6.39           | -                   | -                 | 0.0995                | 0.0323                      |
| 128 <sup>3</sup>   | $\nu$               | $\chi$            | $\eta$                | $\tau_{cool}$ | $A$  | $\phi_0$ | R    | $t_{tot}$ | $t_{turn}$ | $k_w/k_f$ | Re(Rm)      | Re $_{\omega}$ | $u_{rot,0}/u_{tot}$ | $u_{rot}/u_{tot}$ | $r(t_{turn}^{-1})$    | $r_{\omega}(t_{turn}^{-1})$ |
| M_0A000_128        | $2 \cdot 10^{-4}$   | -                 | $2 \cdot 10^{-4}$     | -             | 0    | 1        | 0.2  | -         | -          | -         | 38.0        | -              | -                   | -                 | -                     | -                           |
| M_0A002_128        | $2 \cdot 10^{-4}$   | -                 | $2 \cdot 10^{-4}$     | -             | 0.02 | 1        | 0.2  | -         | -          | -         | 38.6        | -              | -                   | -                 | -                     | -                           |
| M_0A005_128        | $2 \cdot 10^{-4}$   | -                 | $2 \cdot 10^{-4}$     | -             | 0.05 | 1        | 0.2  | -         | -          | -         | 41.9        | -              | -                   | -                 | -                     | -                           |
| M_0A010_128        | $2 \cdot 10^{-4}$   | -                 | $2 \cdot 10^{-4}$     | -             | 0.10 | 1        | 0.2  | -         | -          | -         | 52.1        | -              | -                   | -                 | ND                    | ND                          |
| M_0A020_128        | $2 \cdot 10^{-4}$   | -                 | $2 \cdot 10^{-4}$     | -             | 0.20 | 1        | 0.2  | -         | 0.62       | 0.092     | 80.2        | 7.37           | 0.78                | 0.81              | 0.0296                | 0.00983                     |
| M_0A050_128        | $2 \cdot 10^{-4}$   | -                 | $2 \cdot 10^{-4}$     | -             | 0.50 | 1        | 0.2  | -         | -          | -         | 180.3       | -              | -                   | -                 | ND                    | ND                          |
| M_0A100_128        | $2 \cdot 10^{-4}$   | -                 | $2 \cdot 10^{-4}$     | -             | 1.00 | 1        | 0.2  | -         | -          | -         | 355.1       | -              | -                   | -                 | ND                    | ND                          |
| M_0A020_W0.10_128  | $2 \cdot 10^{-4}$   | -                 | $2 \cdot 10^{-4}$     | -             | 0.20 | 1        | 0.1  | -         | -          | -         | 36.1        | -              | -                   | -                 | -                     | -                           |
| M_0A020_W0.15_128  | $2 \cdot 10^{-4}$   | -                 | $2 \cdot 10^{-4}$     | -             | 0.20 | 1        | 0.15 | -         | 0.50       | 0.071     | 56.6        | 4.01           | 0.87                | 0.91              | 0.0286                | 0.00918                     |
| M_0A020_W0.25_128  | $2 \cdot 10^{-4}$   | -                 | $2 \cdot 10^{-4}$     | -             | 0.20 | 1        | 0.25 | -         | 0.74       | 0.112     | 104.9       | 11.76          | 0.73                | 0.76              | 0.0235                | 0.00853                     |
| M_0A020_F0_128     | $2 \cdot 10^{-4}$   | -                 | $2 \cdot 10^{-4}$     | -             | 0.20 | 0        | -    | -         | -          | -         | 70.5        | -              | -                   | -                 | -                     | -                           |
| M_0A020_F0.5_128   | $2 \cdot 10^{-4}$   | -                 | $2 \cdot 10^{-4}$     | -             | 0.20 | 0.5      | 0.2  | -         | 0.68       | 0.096     | 74.1        | 7.10           | 0.91                | 0.92              | 0.0290                | 0.00875                     |
| M_0A020_F1.5_128   | $2 \cdot 10^{-4}$   | -                 | $2 \cdot 10^{-4}$     | -             | 0.20 | 1.5      | 0.2  | -         | 0.58       | 0.099     | 85.8        | 8.49           | 0.70                | 0.75              | 0.0239                | 0.00857                     |
| 256 <sup>3</sup>   | $\nu$               | $\chi$            | $\eta$                | $\tau_{cool}$ | $A$  | $\phi_0$ | R    | $t_{tot}$ | $t_{turn}$ | $k_w/k_f$ | Re(Rm)      | Re $_{\omega}$ | $u_{rot,0}/u_{tot}$ | $u_{rot}/u_{tot}$ | $r(t_{turn}^{-1})$    | $r_{\omega}(t_{turn}^{-1})$ |
| M_0A010            | $2 \cdot 10^{-4}$   | -                 | $2 \cdot 10^{-4}$     | -             | 0.10 | 1        | 0.2  | -         | 1.00       | 0.073     | 49.8        | 3.61           | 0.51                | 0.68              | 0.0155                | 0.00756                     |
| M_0A015            | $2 \cdot 10^{-4}$   | -                 | $2 \cdot 10^{-4}$     | -             | 0.15 | 1        | 0.2  | -         | 0.79       | 0.085     | 63.5        | 5.40           | 0.70                | 0.76              | 0.0220                | 0.00944                     |
| H_0A020            | $2 \cdot 10^{-4}$   | -                 | -                     | -             | 0.20 | 1        | 0.2  | -         | -          | - 78.9    | -           | -              | -                   | -                 | -                     | -                           |
| M_0A020            | $2 \cdot 10^{-4}$   | -                 | $2 \cdot 10^{-4}$     | -             | 0.20 | 1        | 0.2  | -         | 0.63       | 0.091     | 78.9        | 7.19           | 0.81                | 0.86              | 0.0262                | 0.00969                     |
| MB_0A020           | $2 \cdot 10^{-4}$   | $2 \cdot 10^{-4}$ | $2 \cdot 10^{-4}$     | -             | 0.50 | 1        | 0.2  | -         | 0.65       | 0.093     | 76.9        | 7.15           | 0.85                | 0.88              | 0.0316                | 0.00925                     |
| M_0A050            | $2 \cdot 10^{-4}$   | -                 | $2 \cdot 10^{-4}$     | -             | 0.50 | 1        | 0.2  | -         | 0.28       | 0.103     | 181.1       | 18.74          | 0.96                | 0.97              | 0.0510                | 0.0143                      |
